# Supplementary material for: Ising Meson Spectroscopy on a Noisy Digital Quantum Simulator
Source: arXiv:2303.03311 source file (2024-06-10)
Supplement: Supplementary file 1 [file suppl.pdf]

# Supplementary Materials: Ising Meson Spectroscopy on a Noisy Digital Quantum Simulator

Christopher Lamb,<sup>\*</sup> Yicheng Tang, Robert Davis, and Ananda Roy<sup>†</sup>

*Department of Physics and Astronomy, Rutgers University, Piscataway, NJ 08854-8019 USA*

The supplementary material is organized as follows. In Sec. I, details of the experimental implementation are provided together with additional data used in the main text of the manuscript. Sec. II outlines a corresponding experimental protocol for the XY chain in the presence of a longitudinal field. For the XY model, noiseless Qiskit simulations and comparison with exact computations are provided.

## I. EXPERIMENT SETUP, IMPLEMENTATION AND ADDITIONAL DATA

The experiment is set up by initializing the state  $|\rightarrow, \dots, \rightarrow\rangle$  by applying a Hadamard gate to each qubit in the  $|0, \dots, 0\rangle$  ground state. A unitary comprised of the trotterized time evolution of the Hamiltonian is applied for each  $\Delta t$ . After each Trotter step, all the qubits are measured.

We implement the quench protocol by a Trotter decomposition of the time evolution for the Hamiltonian:

$$H = - \sum_{j=0}^{L-1} (\sigma_j^x \sigma_{j+1}^x + g \sigma_j^z + h \sigma_j^x)$$

$$e^{-iHt} = e^{-i(H_{xx} + H_z + H_x)t} \approx \prod_1^n e^{-iH_{xx}\delta t} e^{-iH_z\delta t} e^{-iH_x\delta t}$$

where  $H_{xx} = -J \sum_j X_j X_{j+1}$ ,  $H_z = -g \sum_j Z_j$ , and  $H_x = -h \sum_j X_j$ . The unitary was decomposed further by changing the single qubit gates to the second-order Trotter decomposition while leaving the two-qubit rotation gates as first order.

$$e^{-iHt} \approx \prod_1^n e^{-iH_x \frac{\delta t}{2}} e^{-iH_z \frac{\delta t}{2}} e^{-iH_{xx}\delta t} e^{-iH_z \frac{\delta t}{2}} e^{-iH_x \frac{\delta t}{2}}$$

$$e^{-iH_{xx}\delta t} \rightarrow R_{xx}(-2J\delta t)$$

$$e^{-iH_z\delta t} \rightarrow R_z(-g\delta t)$$

$$e^{-iH_x\delta t} \rightarrow R_x(-h\delta t)$$

The two-qubit rotation gate,  $R_{xx}$ , was applied to the even and odd qubit indices to run as many operations in parallel as possible. Running the gates in parallel shortened the overall depth of the circuit to execute more gates during the qubit lifetimes.

To run the circuits on `ibmq_mumbai`, which has IBM's 27-qubit Falcon processor, the circuit needed to be transpiled for the qubits to map to the qubit loops available on the processor. This was done by passing in the initial layout of numbered qubits that correspond to available chains from the connectivity graphs. When the circuits were being transpiled, we added dynamical decoupling [1] by setting the optimization level to 3. Dynamical decoupling is a class of error mitigation techniques that add spin echoes to the transpiled circuits. The spin echoes send pulses to idle qubits returning the qubits to their original states and undoing potentially adverse effects from nearby qubits.

---

<sup>\*</sup> cdl92@physics.rutgers.edu

<sup>†</sup> ananda.roy@physics.rutgers.edu

The circuits were executed using the qiskit runtime primitive, Sampler. Using Sampler, we applied Twirled readout error extinction (T-REx) [2] to our circuits by setting the resilience level to 1 in the run options. T-REx uses an error mitigation technique known as Pauli twirling to reduce the noise from the measurement by comparing the zero state results with the noisy results with randomized bit flips added to each set of results.

When the executed jobs returned, the magnetization was calculated by taking the quasi-probabilities and converting them to the binary probabilities, then using the marginal counts to get the magnetization for each of the measured qubits for each time step.

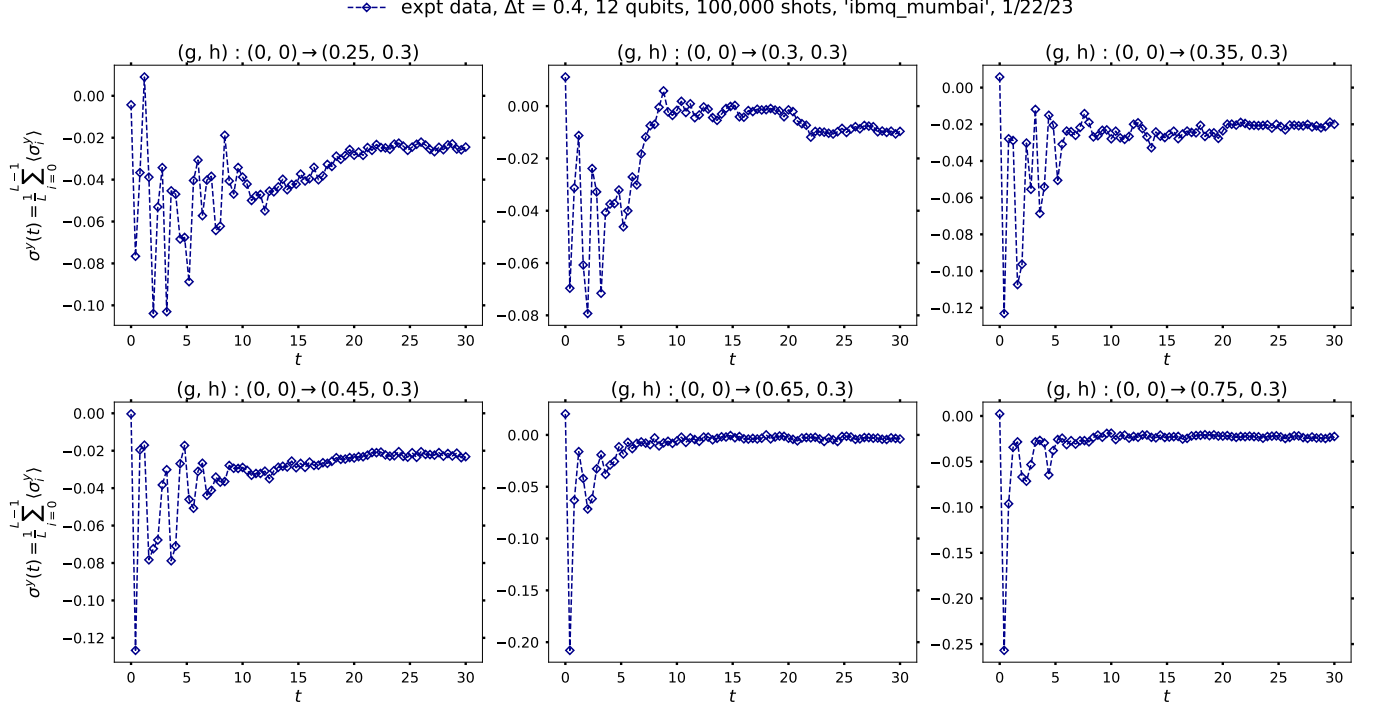

FIG. 1. Experimental results for the measurement of  $\sigma^y(t)$  quenches from  $g = h = 0$ . The Qiskit twirled readout error extinction and dynamical decoupling schemes were used to mitigate the effects of noise present in the IBM Mumbai simulator. These data are analyzed for Fig. 2 and 3 of the maintext (see corresponding figures for further details). Dashed blue lines are meant to be a guide for the eye.

## II. THE XY MODEL IN THE PRESENCE OF A LONGITUDINAL FIELD

We start with the model that describes the quantum sine-Gordon model perturbed by a cosine potential with twice the periodicity in the free-fermion limit, which is governed by the lattice Hamiltonian:

$$H = - \sum_{i=0}^{N-1} (J_x \sigma_i^x \sigma_{i+1}^x + J_y \sigma_i^y \sigma_{i+1}^y) - \sum_{i=0}^{N-1} h_x \sigma_i^x,$$

with periodic boundary conditions. The similar mesonic state spectrum as in the Ising case we studied can be observed after a global quench.

The quench protocol comprises the following steps:

1. *Initial state preparation:* The system is prepared in the ground state of the Hamiltonian with  $h = 0, 0 \leq J_y$ . In this work, we will restrict to initial product states:  $|\psi_0\rangle = |\rightarrow\rangle^{\otimes L}$ , i.e., the case  $J_y = 0, h = 0$ , due to the simplicity of implementation on a quantum simulator. In this case, the initial state is prepared by simply applying a Hadamard gate on the canonical ground state of each spin.
2. *Trotterized time-evolution:* A global quench is performed to  $h > 0$  with or without changing  $\kappa$ . The unitary evolution operator:  $U = e^{-iHt}$  can be implemented on a classical computer either as a whole in exact simulations

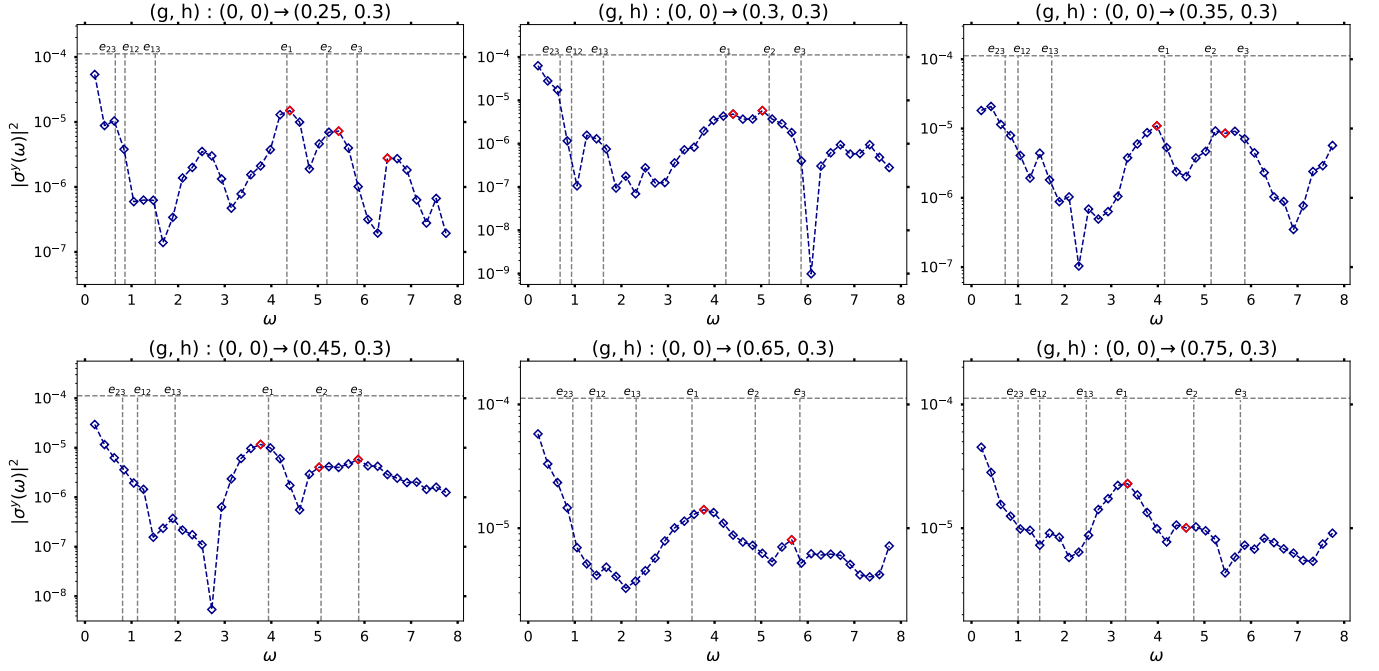

FIG. 2. Absolute value of the Fourier transforms of the data shown in Fig. 2. The different meson rest energies are obtained by locating the maxima in the corresponding data (red markers). Dashed blue lines are a guide for the eye.

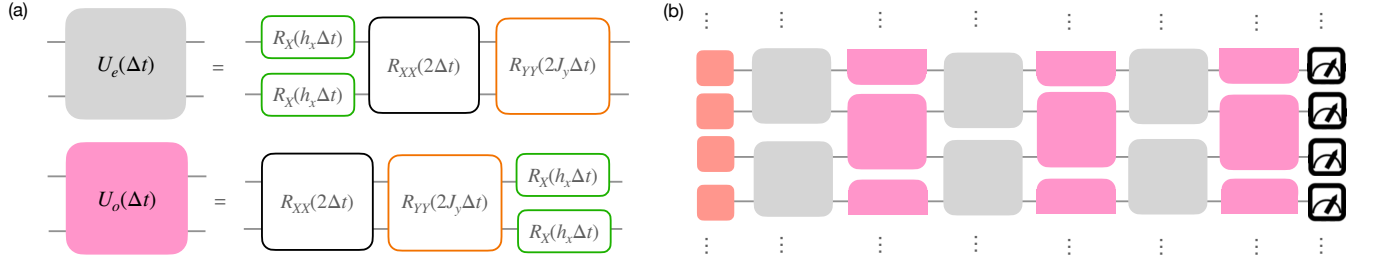

FIG. 3. (a) The decompositions of  $U_e$  and  $U_o$  in terms of single and two-qubit gates are shown. (b) Schematic of the trotterized unitary time-evolution generated by the Hamiltonian  $H$ . The action of the full unitary operator is decomposed into the unitary operators:  $U_e$  and  $U_o$ . At the end of the time-evolution, single qubit measurements are performed on the  $\sigma^x$  basis.

or as a sequence of two-site unitary operations in tensor-network computations, as shown in Fig. 3. For a quantum simulator, the unitary operator is decomposed into single and two-qubit gates, see below for more details.

3. *Measurement of observables:* It turns out that measurement of single-spin operators,  $\sigma_j^\alpha$ ,  $\alpha = x, y, z$ , are already sufficient to compute the meson masses [3]. These measurements are straightforward to implement on a quantum simulator. The results are shown in Fig. 4. Spin correlation functions can be computed directly from these measurement results. These contain signatures of the confinement phenomena occurring in the spin chains.

### A. Meson Energy in Zero Momentum Sector

To get the static mesonic state, we want to diagonalize the Hamiltonian in the zero momentum sector (see, for example, Ref. [4] for details). By writing the states in the  $\sigma^x$  basis as  $|s_0, s_1, \dots, s_{N-1}\rangle$ , with  $s_i = 0$  or 1. Thus a binary number from 0 to  $2^N - 1$  can represent a basis without ambiguity. The transfer operator  $T = e^{ipa}$  acts as  $T|s_0, s_1, \dots, s_{N-1}\rangle = |s_1, s_2, \dots, s_{N-1}, s_0\rangle$ . Thus a translational invariant state is defined as  $T|\psi\rangle = |\psi\rangle$ .

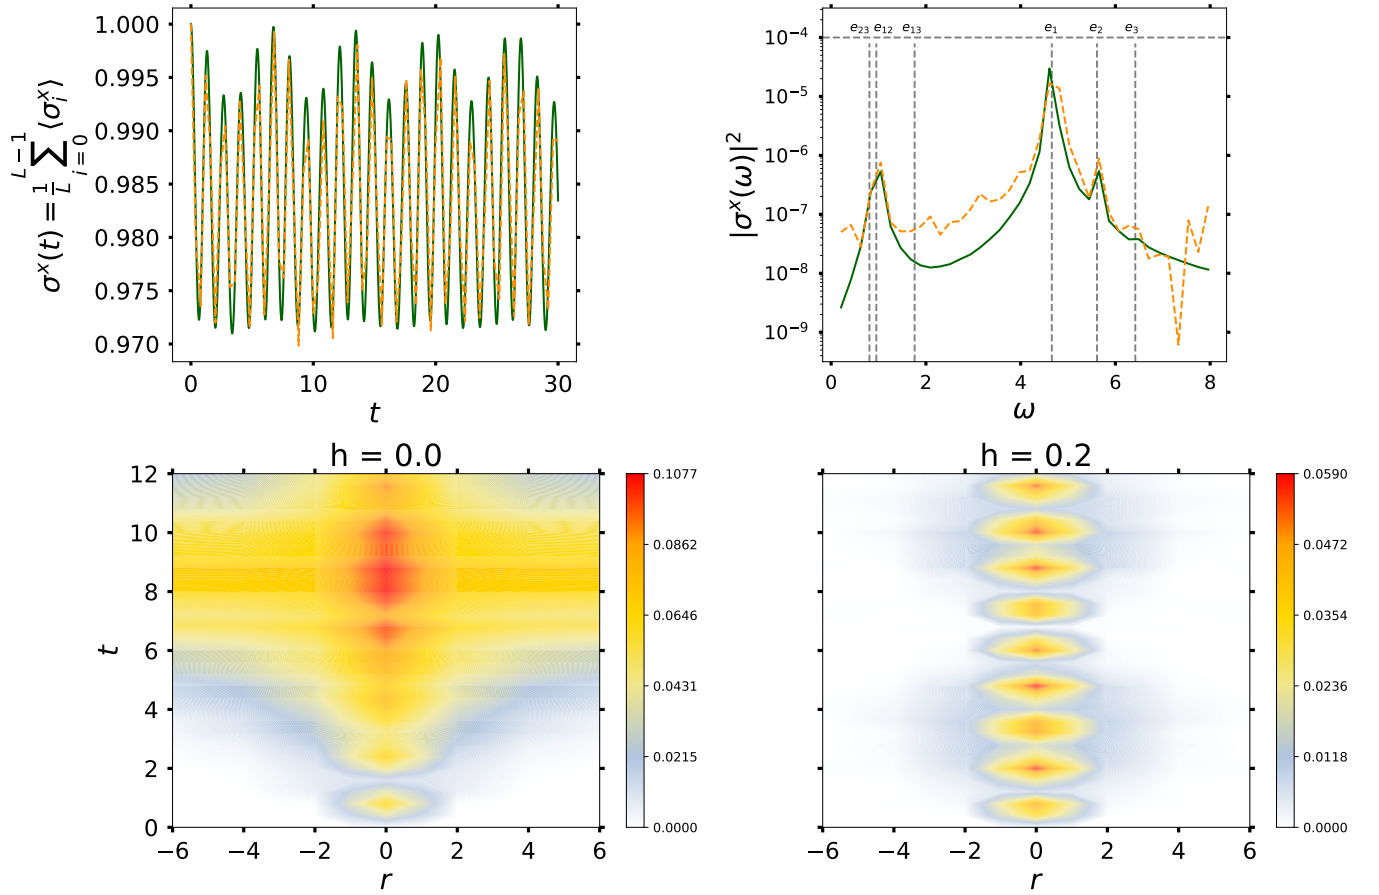

FIG. 4. (Top panels) Measurement results for  $\sigma^x(t)$  and its Fourier transform  $\sigma^x(\omega)$  after the quench with parameter  $Jy = 0.2$  and  $h_x = 0.2$ . The dashed lines are meson mass calculated from exact diagonalization. The results obtained using an exact simulation of the time evolution of  $L = 12$  qubits with  $\Delta t = 0.01$  are shown with green solid lines. The noiseless numerical Qiskit simulation results are performed for  $\Delta t = 0.4$  (orange dashed line). The peaks in the latter correspond to the rest energies ( $e_n$ ), of the mesonic excitations labeled by  $n$ , and their differences ( $e_{mn}$ ). The gray dashed lines correspond to the exact diagonalization results obtained in the zero momentum sector. (Bottom panels) Measurement results for the correlation function  $G_x(r, t) = \langle \sigma_i^x(t) \sigma_{i+r}^x(t) \rangle - \langle \sigma_i^x(t) \rangle \langle \sigma_{i+r}^x(t) \rangle$ . The presence of the magnetic field clearly leads to the confinement of the domain wall excitations.

For an arbitrary basis vector  $|a\rangle = |s_0, s_1, \dots, s_{N-1}\rangle$ , then  $|\bar{a}\rangle = \sum_{n=0}^{N-1} T^n |a\rangle$  must be a translational invariant state. Defining an equivalent class such that if  $|a\rangle = T^l |b\rangle$ , then  $|a\rangle$  and  $|b\rangle$  are equivalent,  $|\bar{a}\rangle$  from each class forms a complete basis for the zero momentum sector. The size of this equivalent class  $p(a)$  is called the period since  $T^p |a\rangle = |a\rangle$ .

Using the translational symmetry, the matrix element of the Hamiltonian can be calculated as

$$H_{ab} = \langle \bar{b} | H | \bar{a} \rangle = \sqrt{\frac{p(a)}{p(b)}} \langle a | H | b \rangle. \quad (1)$$

Thus after finding all the matrix elements in the zero momentum sector, one can diagonalize the Hamiltonian. After diagonalizing the Hamiltonian in the zero-momentum sector, we calculated the energy  $E_n = \langle n | H | n \rangle$  for all the eigenvectors  $|n\rangle$ .

- 
- [1] L. Viola and S. Lloyd, Dynamical suppression of decoherence in two-state quantum systems, *Phys. Rev. A* **58**, 2733 (1998).  
 [2] E. van den Berg, Z. K. Mineev, and K. Temme, Model-free readout-error mitigation for quantum expectation values, *Phys. Rev. A* **105**, 032620 (2022).

- [3] M. Kormos, M. Collura, G. Takács, and P. Calabrese, Real-time confinement following a quantum quench to a non-integrable model, [Nature Physics](#) **13**, 246 (2016).
- [4] A. W. Sandvik, Computational Studies of Quantum Spin Systems, [AIP Conf. Proc.](#) **1297**, 135 (2010), [arXiv:1101.3281 \[cond-mat.str-el\]](#).
